# Supplementary material for: A Survey on Autonomous Driving Datasets: Statistics, Annotation Quality, and a Future Outlook
Source: arXiv:2401.01454 source file (2024-04-23)
Supplement: Supplementary file 1 [file supplementary.tex]

\documentclass[lettersize,journal]{IEEEtran}
\usepackage{amsmath,amsfonts}
\usepackage{algorithmic}
\usepackage{algorithm}
\usepackage{array}
\usepackage{textcomp}
\usepackage{stfloats}
\usepackage{url}
\usepackage{verbatim}
\usepackage{graphicx}
\usepackage{cite}
\usepackage{multicol}
\usepackage{multirow}
\usepackage{tabularx}
\usepackage{booktabs}
\usepackage{bbding}
\usepackage{subfigure}
\usepackage{colortbl}
\usepackage{graphicx}
\usepackage{svg}
\usepackage{hyperref}
\usepackage{footnote}
\usepackage{orcidlink}
\hypersetup{
    colorlinks=true,
    linkcolor=red,
    urlcolor=red
}

\hyphenation{op-tical net-works semi-conduc-tor IEEE-Xplore}
% updated with editorial comments 8/9/2021

\begin{document}

% \title{A Survey on Autonomous Driving Datasets: Statistics, Annotation, and Outlook}
% \title{A Survey on Autonomous Driving Datasets: Statistics, Annotation Quality, and a Future Outlook}
% \title{A Survey on Autonomous Driving Datasets: Statistics, Annotation Quality, and a Future Outlook}

% \maketitle

\input{tables_images/all_datasets}
\input{tables_images/all_datasets2}

\clearpage
% ========= Reference ========== %
{
    % \small
    \bibliographystyle{ieeetr}
    \bibliography{reference}
}

\end{document}
